# Supplementary material for: MagicClay: Sculpting Meshes With Generative Neural Fields
Source: arXiv:2403.02460 source file (2024-10-09)
Supplement: Supplementary file 1 [file appendix.tex]

\section{Additional Related Work}

\paragraph{{\bf Mesh optimizations with topology updates}} While it's relatively easy to optimize the position of vertices in a mesh via gradient descent, it's  notoriously hard to optimize  the triangulation, the number of triangles and the number of vertices because these are discrete properties. 
 Point2mesh ~\cite{point2mesh2020} optimizes a mesh to fit a point cloud using a course-to-fine approach, where after each stage a remeshing algorithm \cite{botschRemesh2004} is applied. Nicolet \etal~\cite{largesteps2021} uses differentiable rendering to optimize the vertices, with \cite{botschRemesh2004} applied periodically to decrease the average edge length by half the current value.   Palfinger~\cite{continous_remshing2022} proposes a Continous Remeshing approach, where local topology edits are performed at every iteration, guided by the Adam optimizer's vertex speeds. %To facilitate this, these local topology edits are implemented using the GPU. 
 ROAR~\cite{barda2023roar} improves the adaptivity of the continous remeshing approach by decoupling the local topology editing from the noisy Adam parameters and defining a face curvature score using mesh supersampling and projection operators. This curvature score guides the local topology edits, and allows achieving sparser meshes. \ourmethod{} performs topology updates using ROAR. While Nicolet ~\etal~\cite{largesteps2021}, ROAR~\cite{barda2023roar} and Continuous Remeshing~\cite{continous_remshing2022} showcase their method via a multi-view reconstruction task, the sculpting problem we tackle is generative, and the optimization gradients can be very noisy. On this task, we compare against Continuous Remeshing equipped with Score-Distillation Sampling gradients, and empirically show the importance of using ROAR on our hybrid representation.
