# Supplementary material for: MagicClay: Sculpting Meshes With Generative Neural Fields
Source: arXiv:2403.02460 source file (2024-10-09)
Supplement: Supplementary file 3 [file quantitative_results_uncond_detailed_suppmat.tex]

\begin{table*}[t]
\begin{tabular}{|l|l|l|l|l|l|l|l|l|l|l|l|}
 &  P1$\uparrow$ &  P2 $\uparrow$ &  P3 $\uparrow$ &  P4 $\uparrow$ &  P5 $\uparrow$ &  P6 $\uparrow$ &  P7 $\uparrow$ &  P8 $\uparrow$ &  P9 $\uparrow$ &  P10 $\uparrow$ & mean $\uparrow$ \\
 \hline
 Fantasia3D (Mesh) &  23.73&  22.62&  25.54&  20.06&  25.88&  22.69&  26.81&  22.47&  25.01&  24.84 &23.97
\\
 \hline
 ProlificDreamer (NeRF)&  22.22&  21.54&  22.51&  21.35& 22.87 &  21.8&  16.65&  20.26&  23.33& ?? &21.21
 \\
 
 ProlificDreamer (Mesh)& 22.82  & 20.11 & 19.46  & 20.89 & 20.94 & 21.53 & 14.4 & 19.7  & 21.6 & 19.46 & 20.06 \\
  \hline
 Hifa (NeRF) & 27.43 & 20.46 & 24.17 & 20.46 & 20.81 & 19.59 & 22.09 & 24.56 & 26.55  & 25.22 & 23.16 \\
 
 Hifa (Mesh) & 26.67 & 17.13 & 22.04 & 20.38 & 19.74 & 19.35 & 19.33 & 24.41 & 26.79  & 24.84 & 22.01 \\
\hline
 TextMesh (SDF) & 24.11 & 22.17 & 28.65 & 21.13  & 24.79 & 22.61 & 27.68 & 27.38 & 25.63 & 25.23 & 24.92 \\
  TextMesh (Mesh) & 28.69 & 20.0 & 25.23 & 20.52 & 21.54 & 21.56 & 23.86 & 24.53 & 24.09 & 22.59 & 23.56 \\
  \hline
   MVDreams (NeRF) & 25.42 & 25.29 & 23.39 & 25.34 & 25.14 & 26.08 & 27.51 &  & 24.98 & 26.67 & 25.43 \\
   MVDreams (Mesh) & 23.59 & 24.95 & 22.45 &  & 24.56 & 26.92 & 22.50 & 20.77 & 27.16 & 25.59 & 24.05 \\
  \hline
 ours (SDF) & 24.32 &  &  &  &  &  &  &  &  &  &  \\
ours (Mesh) & \textbf{30.7125} &  &  &  &  &  &  &  &  &  &  \\
  \hline
\end{tabular}
\caption{{\bf Quantitative comparison.} \todo{unconditional 3D generation}. We calculate the average clip score for 25 normal renders of the NeRFs/SDFs and meshes for various generative pipelines, taken in a equidistant circular pattern around the generated object. We apply marching cubes to extract the resulting meshes from the NeRFs/SDFs. There is a noticeable drop in the clip score for all single representation pipelines between the renders of the implicit function and the extracted mesh, which can qualitatively be seen in \ref{fig:gen_comparison}. \todo{keep only mean in main paper, put details in sup mat, use 20 prompts). We don't have the drop because we optimize the mesh part as well. Mention clip socre is cosine similarity} }
\end{table*}
